# Supplementary material for: Understanding the origin of superconducting dome in electron-doped MoS$_2$ monolayer
Source: arXiv:2412.02822 ancillary file (2024-12-03)
Supplement: Supplementary file 1 [file SuppInfo.pdf]

# Supplementary information for:
# Understanding the origin of superconducting dome in electron-doped $MoS_2$ monolayer

Nina Girotto Erhardt,[1,*] Jan Berges,[2] Samuel Poncé,[3,4] and Dino Novko[1,†]

[1] *Centre for Advanced Laser Techniques, Institute of Physics, 10000 Zagreb, Croatia*

[2] *U Bremen Excellence Chair, Bremen Center for Computational Materials Science, and MAPEX Center for Materials and Processes, Universität Bremen, 28359 Bremen, Germany*

[3] *European Theoretical Spectroscopy Facility, Institute of Condensed Matter and Nanosciences, Université catholique de Louvain, 1348 Louvain-la-Neuve, Belgium*

[4] *WEL Research Institute, 1300 Wavre, Belgium*

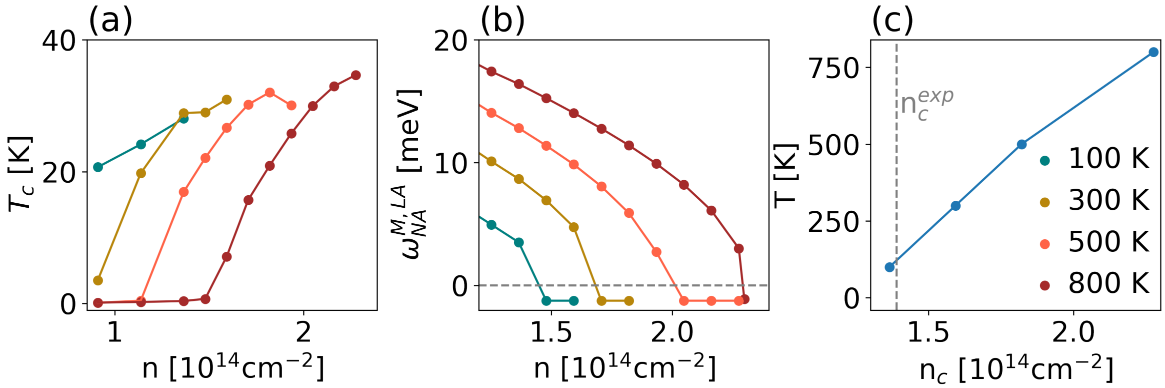


**Supplementary Figure 1**. (a) $T_c$ calculated at various temperatures. (b) Dynamically corrected frequency of the soft $A_1$ mode calculated for various temperatures and dopings. (c) Temperature dependence of the critical doping concentration, for which the $T_c$ shows the maximum (top of the dome structure). The dashed line shows the experimental value for the critical concentration. In the low-doping $1 \times 1$ H phase we investigated how the value of $T_c$ depends on the temperature at which the dynamical effects of EPC are calculated. In panel (a) we observe that a reduction in temperature results in shifting the superconducting onset to lower dopings, closer to the experimental values, as well as in a slight decrease of the $T_c$ value. It is important to note that a change in temperature was imposed in EPW, while the starting point for all the presented temperatures was a DFPT calculation with a smearing value corresponding to 800 K. Therefore, the static phonon self-energy at 800 K was first subtracted from the DFPT frequencies, and after that a dynamic self-energy at a desired temperature was added. The results also show how the critical doping value for which the $1 \times 1$ H phase becomes dynamically unstable decreases with temperature. We show the values of dynamically corrected frequencies because the change in temperature is done at the EPW level.

* ngirotto@ifs.hr

† dino.novko@gmail.com

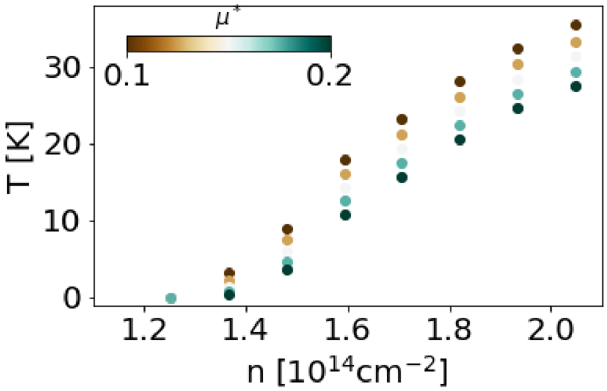


**Supplementary Figure 2**. $T_c$ calculated for various values of $\mu^*$. Value of $T_c$ can be slightly manipulated by the choice of $\mu^*$. Varying the $\mu^*$ parameter from 0.1 to 0.2 changes the calculated $T_c$ value by 10 K.

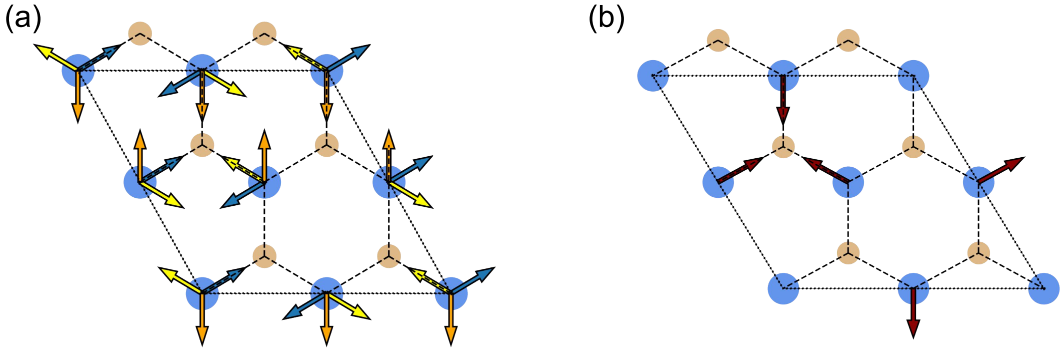


**Supplementary Figure 3**. (a) Schematic representation of the displacements corresponding to the soft $A_1$ (M) phonon in the three inequivalent M points of the Brillouin zone. (b) Superposition of the modes in (a), representing the displacement pattern in the CDW phase.

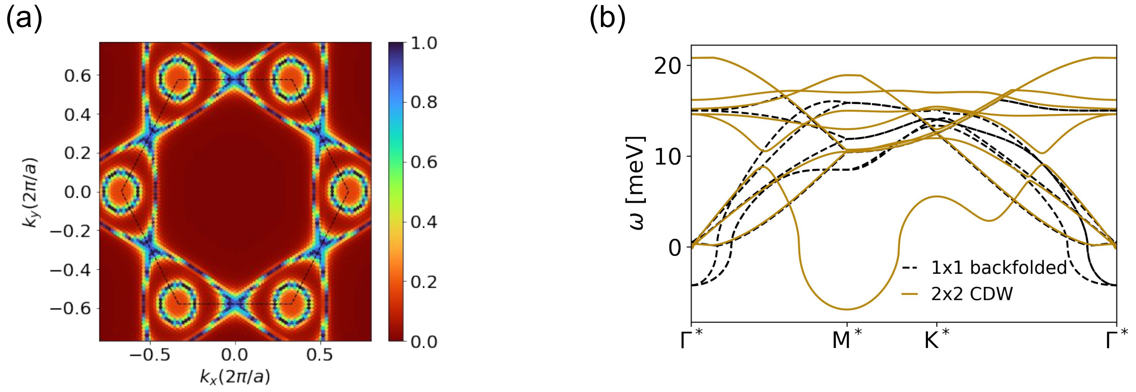


**Supplementary Figure 4**. (a) Fermi surface and a Van Hove singularity of the $2 \times 2$ CDW phase in the unstable region. (b) Corresponding phonon dispersion in comparison with the one for the $1 \times 1$ H structure for the same doping ($n = 2.4 \times 10^{14}\,\mathrm{cm}^{-2}$). Both band structures are plotted inside the smaller $2 \times 2$ BZ, which is why the $1 \times 1$ H phonon instability occurs in the $\Gamma$ point. It is surprising that after the M point instability, a $2 \times 2$ CDW phase is not stabilized. The expected behavior would be the backfolding of the unstable M points to the $\Gamma$, and subsequent relaxation into a new stable structure ($2 \times 2$ CDW), which stabilizes the unstable $\Gamma$ mode. While this is exactly what happens for dopings larger than $2.38 \times 10^{14}\,\mathrm{cm}^{-2}$, a new instability occurs at the M$^*$ point. As one of the possible explanations for this, we propose a Van Hove singularity at the Fermi level in the $2 \times 2$ CDW phase which causes a large DOS. The length of the flat portions of the Fermi surface is equal to the distance between the $\Gamma$ and M$^*$ points. Therefore, $\mathbf{q} = \mathrm{M}^*$ wavevector connects the parts with the largest number of carriers causing the instability.

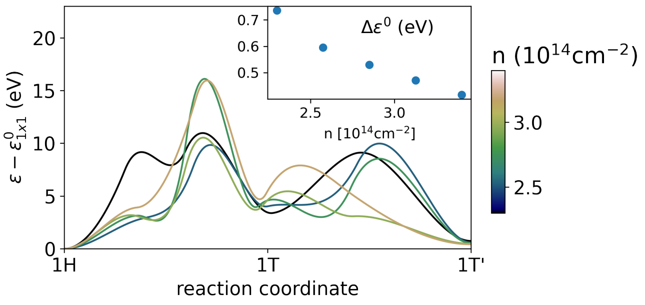


**Supplementary Figure 5**. Doping-dependent potential energy surface starting from a $1 \times 1$ H phase, and finishing at 1T$'$ phase with a 1T phase in the middle. We use the nudged elastic band method, which finds a minimum energy path.

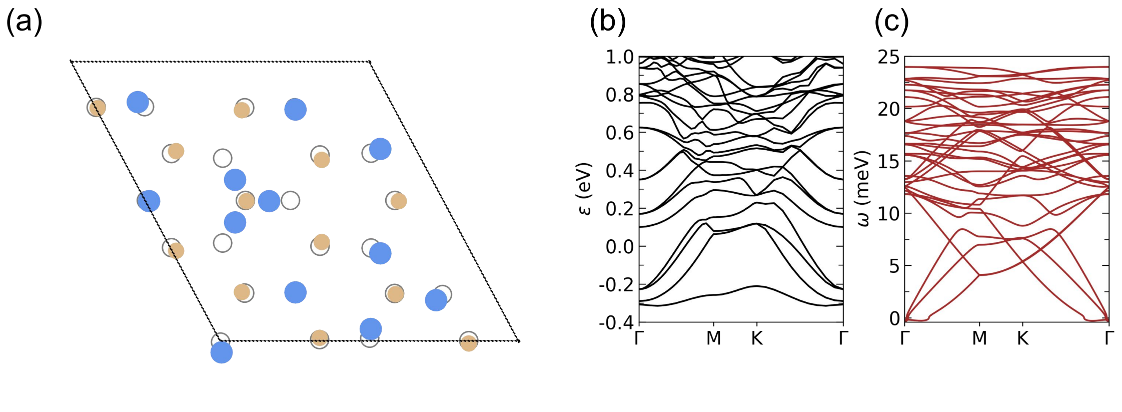


**Supplementary Figure 6**. (a) A relaxed $2\sqrt{3} \times 2\sqrt{3}$ CDW structure for $n = 4.74 \times 10^{14}\,\mathrm{cm}^{-2}$, shown with amplified (10 times) atomic displacements, for clarity. Corresponding (b) electron and (c) phonon band structures.

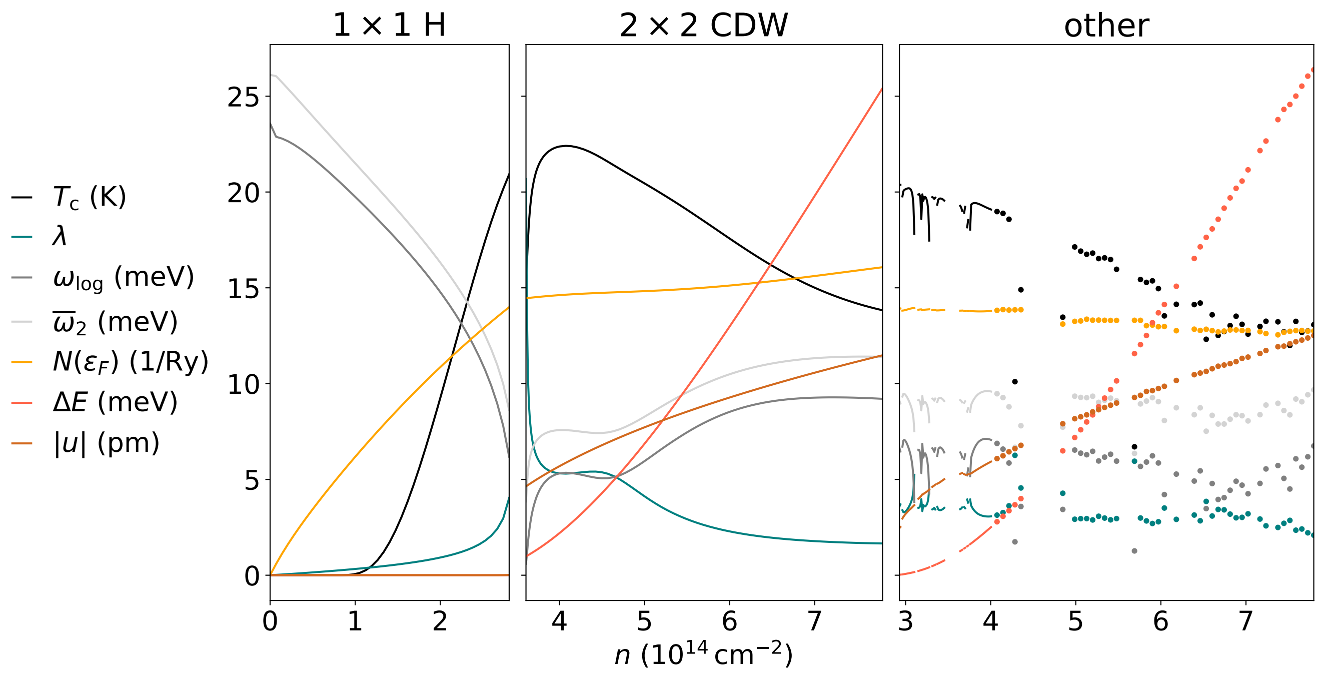


**Supplementary Figure 7**. More detailed characterization of the phases obtained using the model of a linearized, nearest-neighbor electron-phonon coupling. The values for the critical temperature $T_c$ as a function of doping $n$ are reproduced from Fig. 6 of the main text. They have been calculated from the effective electron-phonon interaction $\lambda$, the logarithmic and second-moment average phonon frequencies $\omega_{\log}$ and $\overline{\omega}_2$, and the Coulomb pseudopotential $\mu^* = 0.13$ using the Allen-Dynes formula. Due to the high electronic temperature of $5\,\mathrm{mRy} \approx 800\,\mathrm{K}$, the density of states per spin at the Fermi level $N(\varepsilon_F)$ is smeared and does not show a jump when $\varepsilon_F$ crosses the minimum of the conduction-band valley at $\mathrm{Q} \approx 1/2\,\mathrm{K}$. The energy reduction $\Delta E$ is directly linked to the magnitude of the atomic displacements $|u|$ (vector norm per primitive cell).
